# Supplementary material for: High pressure-temperature phase diagram of ammonia hemihydrate
Source: arXiv:2307.09838 source file (2023-07-19)
Supplement: Supplementary file 1 [file SM_AHH_phase_diagram.pdf]

# Supplementary Material for "High pressure-temperature phase diagram of ammonia hemihydrate"

L. Andriambariarijaona,[1] F. Datchi,[1] H. Zhang,[1] K. Béneut,[1] B. Baptiste,[1] N. Guignot,[2] and S. Ninet[1]

[1]*Institut de Minéralogie, de Physique des Matériaux et de Cosmochimie (IMPMC), Sorbonne Université, CNRS UMR 7590, MNHN, 4, place Jussieu, Paris, France*

[2]*Synchrotron SOLEIL, BP 48, 91192 Gif Sur Yvette, France*

(Dated: July 12, 2023)

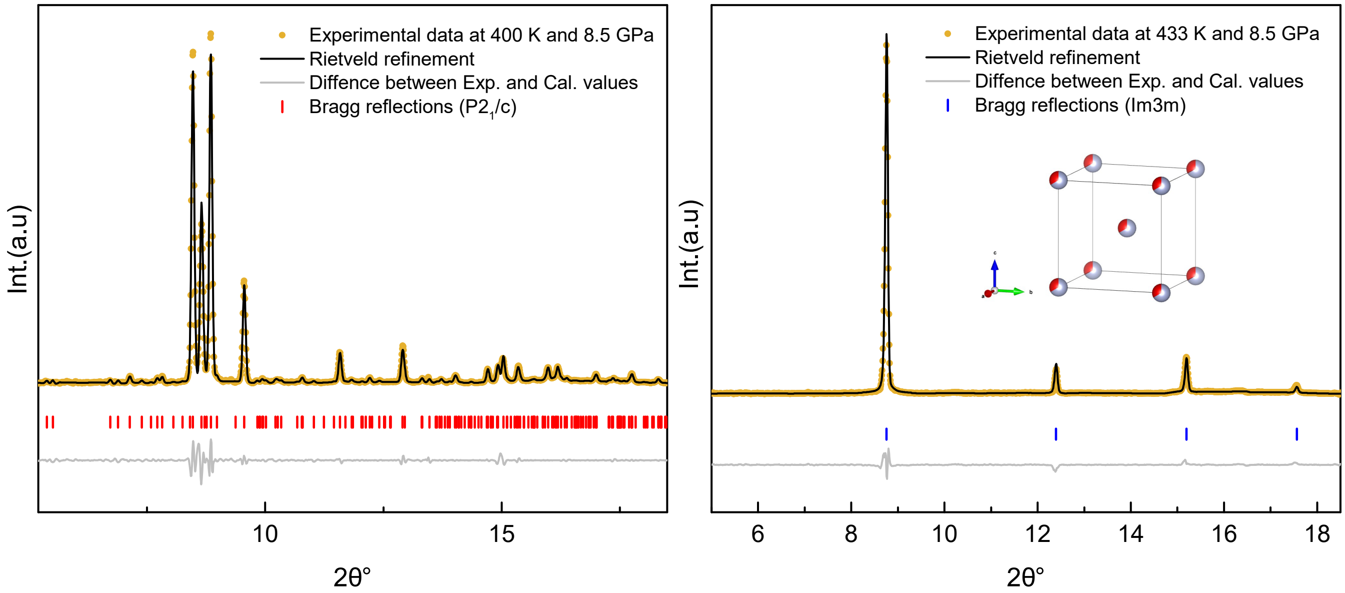


FIG. S1. Rietveld refinement of AHH XRD pattern just below (left) and above (right) the II-*p*bcc transition. The AHH-*p*bcc phase was refined by setting a 1O:2 N occupancy for site (0,0,0) in accordance with the AHH composition, and by ignoring the weak contribution of H atoms.

Table S1. Atomic positions (x,y,z),obtained by Rietveld refinement of the AHH-II structure at 400 K and 8.5 GPa. All atomic sites are on 4e (x,y,z) Wyckoff positions. the lattice parameters are: a = 3.195 Å, b = 8.975 Å, c =8.658 Å and $\beta$ = 94.255 °.

| Atoms | x | y | z |
|---|---|---|---|
| N1 | 0.72554 | 0.11074 | 0.39956 |
| H1 | 0.88697 | -0.02611 | 0.31616 |
| H2 | 0.79294 | 0.14659 | 0.51122 |
| H3 | 0.40650 | 0.09872 | 0.39359 |
| O1 | -0.02823 | 0.88784 | 0.24170 |
| H4 | 0.22231 | 0.70274 | 0.16655 |
| H5 | 0.22716 | 0.92484 | 0.19988 |
| N2 | 1.57538 | 1.84795 | 0.92196 |
| H6 | 0.75256 | 0.88102 | 0.01864 |
| H7 | 0.76918 | 0.80266 | 0.84633 |
| H8 | 0.40994 | 0.93525 | 0.87432 |

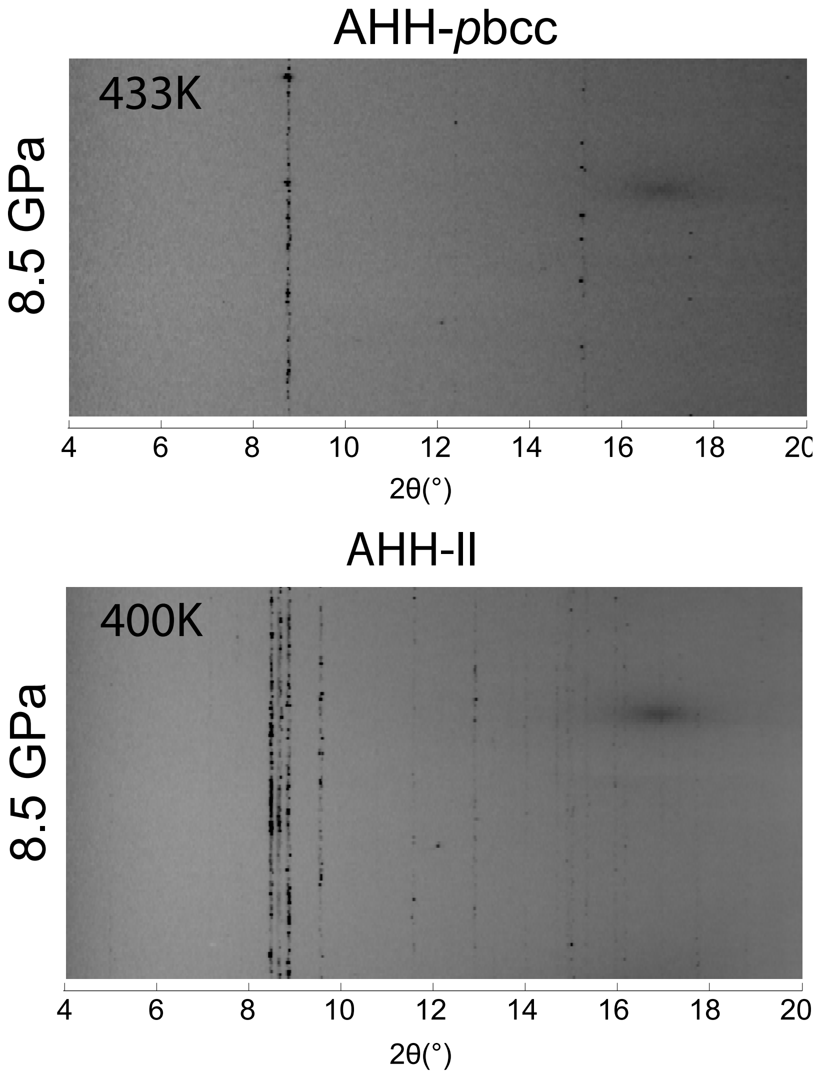


FIG. S2. Cake representation of the x-ray diffraction images of (bottom) AHH-II and (top) AHH-$p$bcc corresponding to the integrated patterns shown in Fig. S1.

Table S2. Lattice parameters of AHH-II (first two lines) and AHH-$p$bcc (last line) resulting from the Rietveld refinement of the experimental data.

| Phase | T(K) | P (GPa) | a (Å) | b (Å) | c (Å) | $\beta$(°) | V (Å$^3$/mol) |
|---|---|---|---|---|---|---|---|
| II | 300 | 6.9 | 3.243 | 9.040 | 8.713 | 94.215 | 21.232(3) |
| II | 400 | 8.5 | 3.195 | 8.975 | 8.658 | 94.255 | 20.628(3) |
| $p$bcc | 433 | 8.5 | 3.463 | 3.463 | 3.463 | 90 | 20.774(3) |

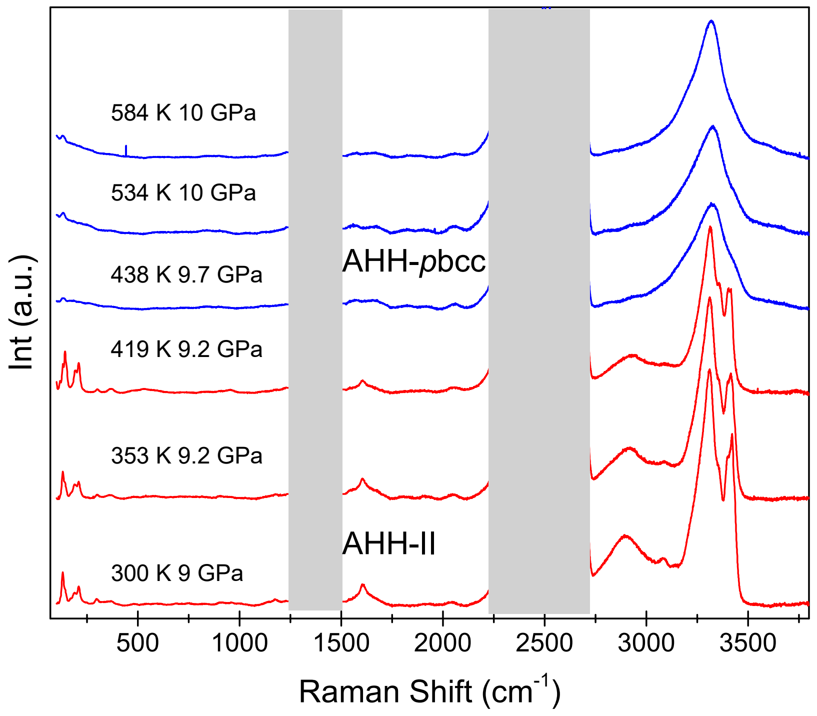


FIG. S3. Evolution of the Raman spectra of a AHH sample as a function of temperature along a quasi-isobaric heating at 9-10 GPa. Red and blue lines are spectra from AHH-II and AHH-*p*bcc, respectively. The frequency windows from 1300-1400 $cm^{-1}$ to 2200 - 2600 $cm^{-1}$ are greyed as they are dominated by, respectively, the first- and second-order Raman signal from the diamond anvils

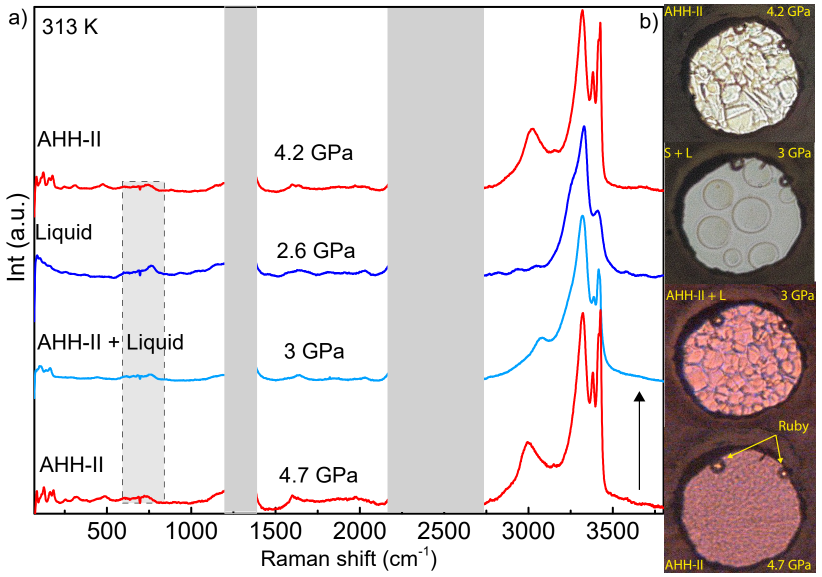


FIG. S4. (a) Evolution of the Raman spectra of AHH during the decompression from 4.7 GPa to 2.6 GPa and then compression to 4.2 GPa at 313 K. The frequency windows from 1200 $cm^{-1}$- 1400 $cm^{-1}$ is grayed as it is dominated by the strong Raman signal from the diamond anvils. The peak around 750 $cm^{-1}$ marked by the dotted frame comes from impurities in the diamond anvils. (b) Photographs of the AHH sample during the same decompression/compression at 313K. The sample composed of AHH-II starts to melt at 3 GPa: the crystalline grains gather and start to move in their liquid while the pressure remains stable. At 2.6 GPa the sample becomes fully fluid. Then, a rapid compression at 4.2 GPa shows that it recrystallizes in the AHH-II phase. Note that the difference in color between the photos is due to different sample illumination conditions, all samples were observed transparent at all conditions.

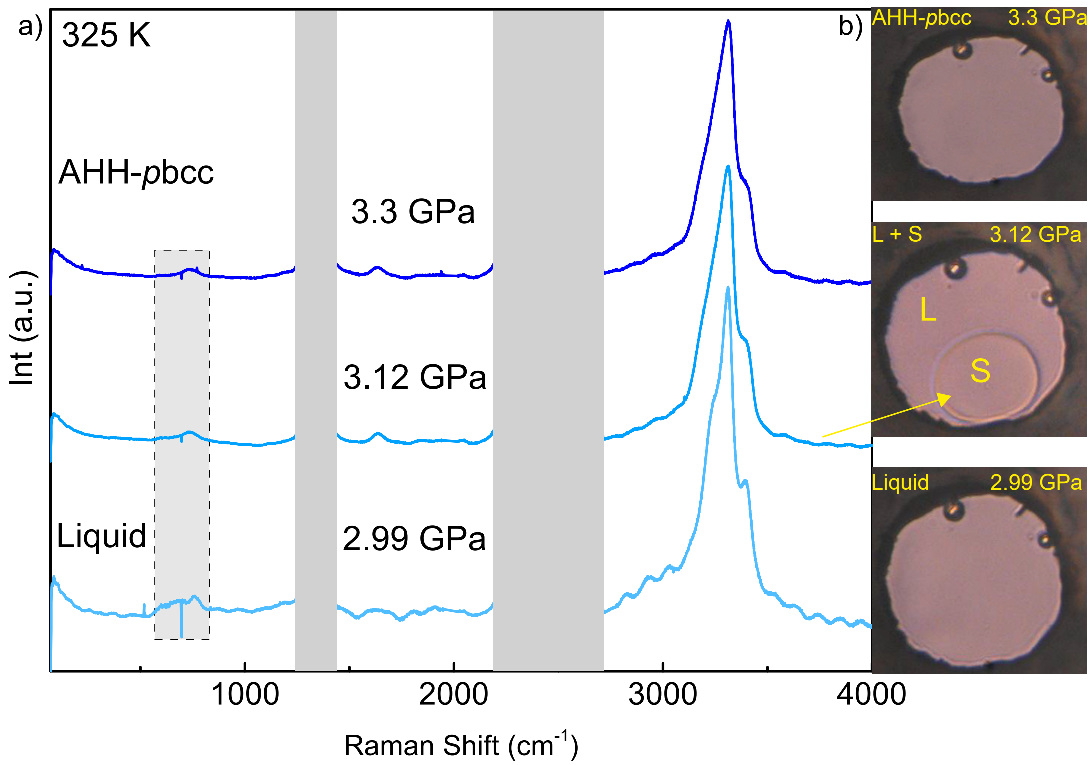


FIG. S5. a)Evolution of the Raman spectra of AHH during Compression from 2.99 GPa to 3.3 GPa at 325 K. The frequency windows from 1300 - 1400 $cm^{-1}$ to 2200 - 2600 $cm^{-1}$ are greyed as they are dominated by, respectively, the first- and second-order Raman signal from the diamond anvils. The peak around 750 $cm^{-1}$ marked by the dotted frame comes from impurities in the diamond anvils.b) Photographs of the AHH sample at the same P-T conditions as the Raman spectra.

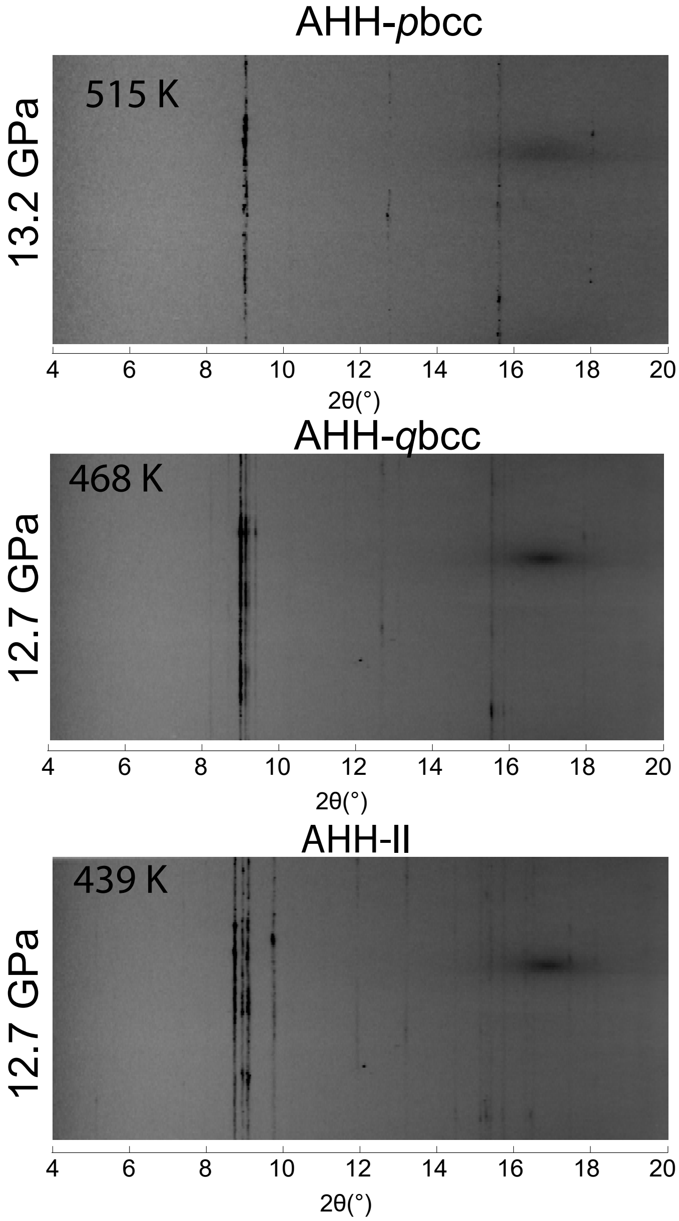


FIG. S6. Cake representation of X-ray powder diffraction pattern measured at the transition between AHH-II ⟶ AHH-$q$bcc and AHH-$q$bcc → AHH-$p$bcc

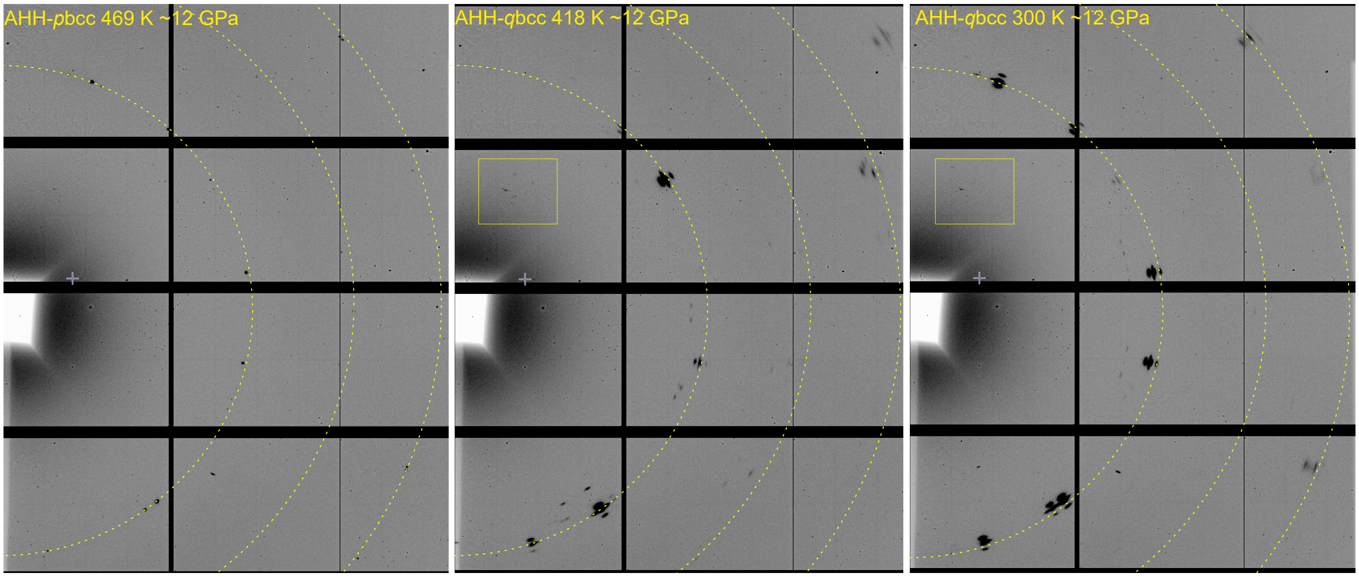


FIG. S7. Diffraction images taken along a quasi isobaric cooling at 12 GPa showing the transition from the $p$bcc to the $q$bcc phase and the recovery of $q$bcc at room temperature. The sample was polycrystalline. The dashed circles are guides for the eyes to indicate the positions of the (110), (200) and (211) reflections of the $p$bcc structure. The boxes show the position of the peaks corresponding to the largest observed intereticular distances (4.52 Å and 3.86 Å) in $q$bcc.

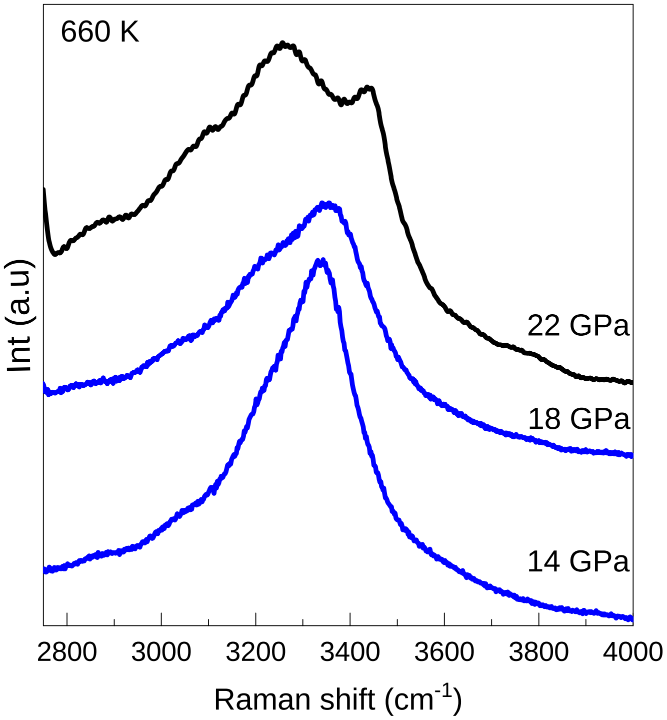


FIG. S8. Evolution of the Raman spectra of AHH along the isotherm at 660 K through the pbcc-DIMA transition. The blue and black spectra correspond to AHH-$p$bcc and AHH-DIMA respectively.

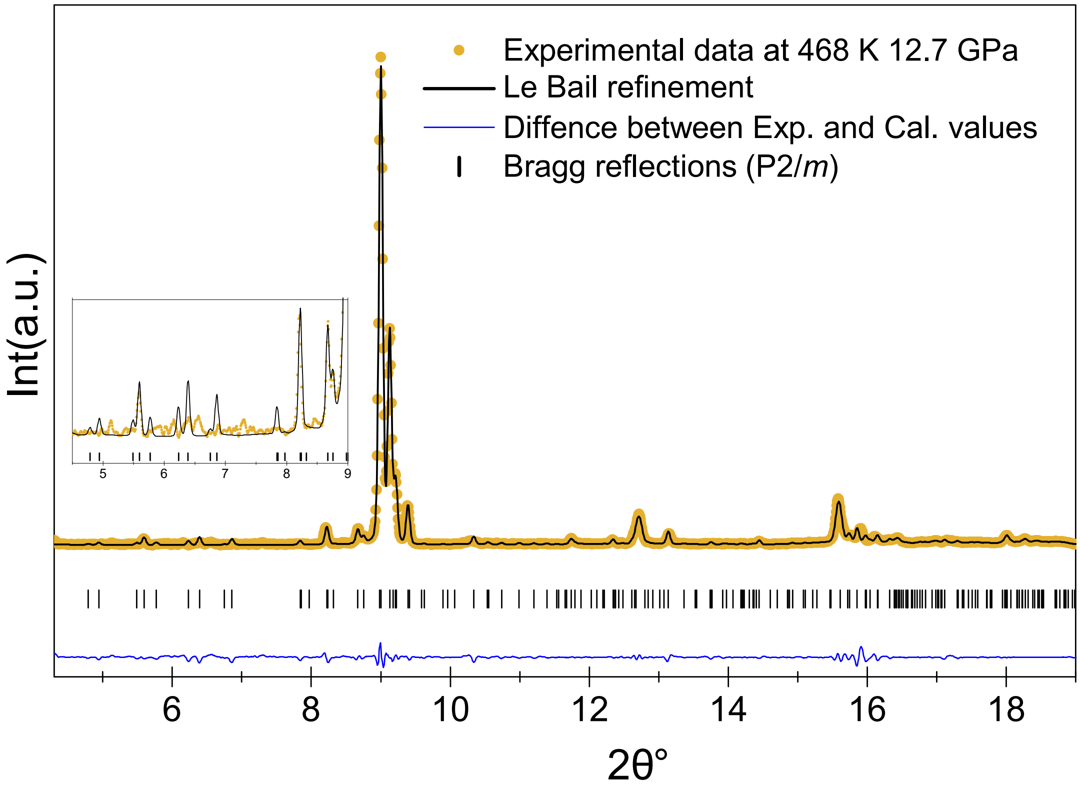


FIG. S9. Le Bail refinement of the AHH-$q$bcc diffractogram to 12.7 GPa, 468 K using the $P2/m$ structure. The symbols are the experimental data and the black line is the refined pattern. The parameters obtained are $a = 5.4606(4)$ Å, $b = 7.8050(3)$ Å, $c = 5.2158(4)$Å and $\beta = 91.78°$. The inset shows a zoom of the low angle peaks from 5 to 9°.
